# Supplementary material for: Learning Perceptual Hallucination for Multi-Robot Navigation in Narrow Hallways
Source: arXiv:2209.13641 source file (2022-09-27)
Supplement: Supplementary file 1 [file appendix.tex]

\section*{APPENDIX}
No Appendix for now. Leave a position for future use.
